# Supplementary material for: Towards QoS-Aware Recommendations
Source: arXiv:1907.06392 source file (2020-10-01)
Supplement: Supplementary file 1 [file AdditionalPlots.tex]

\begin{minipage}[t]{0.46\linewidth}
\includegraphics[width=1\columnwidth]{./figures/figuresSavvas/abandonment.eps}
\label{fig:abandonment}
\includegraphics[width=1\columnwidth]{./figures/figuresSavvas/cdf_interest.eps}
\label{fig:cdf_interest}
\end{minipage}

\begin{minipage}[t]{0.46\linewidth}
\includegraphics[width=1\columnwidth]{./figures/figuresSavvas/cdf_intNext_qorPrev.eps}
\label{fig:cdf_intNext_qorPrev}
\includegraphics[width=1\columnwidth]{./figures/figuresSavvas/chrcrrfixed.eps}
\label{fig:chrcrrfixed}
\end{minipage}

\begin{minipage}[t]{0.46\linewidth}
\includegraphics[width=1\columnwidth]{./figures/figuresSavvas/chrXindex.eps}
\label{fig:chrXindex}
\includegraphics[width=1\columnwidth]{./figures/figuresSavvas/chrXqorXint.eps}
\label{fig:chrXqorXint}
\end{minipage}

\begin{minipage}[t]{0.46\linewidth}
\includegraphics[width=1\columnwidth]{./figures/figuresSavvas/intsoi.eps}
\label{fig:intsoi}
\includegraphics[width=1\columnwidth]{./figures/figuresSavvas/intsoibuckets.eps}
\label{fig:intsoibuckets}
\end{minipage}

\begin{minipage}[t]{0.46\linewidth}
\includegraphics[width=1\columnwidth]{./figures/figuresSavvas/qorsoibuckets.eps}
\label{fig:qorsoibuckets}
\includegraphics[width=1\columnwidth]{./figures/figuresSavvas/qorsoifixed.eps}
\label{fig:qorsoifixed}
\end{minipage}
