# Supplementary material for: Towards QoS-Aware Recommendations
Source: arXiv:1907.06392 source file (2020-10-01)
Supplement: Supplementary file 2 [file Appendix.tex]

\section{ML Results with all samples (no removal of outliers)}

\begin{figure}[h]\centering
\begin{minipage}[t]{\mycustomwidth}
\centering
\includegraphics[width=\mycustomcolumnwidth]{./figures/ML_plots/bestModelHeatmap_diff1.eps}
\caption{ Accuracy of Predictive \textit{QoE} model with +/- 1 distance from true target --no Outliers.}
\label{fig:model-accuracy-diff1}
\end{minipage}
\end{figure}

\begin{figure}
\centering
\subfigure[Num. of Features Used vs. MAE]{\includegraphics[width=\mycustomwidth]{./figures/ML_plots/featureSelection.eps}\label{fig:MAE-vs-nb-features}}
\caption{MAE of Ordinal Regression model vs. number of top features (from Table~\ref{table:weights-ordinal}) used.}
\end{figure}

\begin{table}[h]
\centering
\caption{Mean absolute error, MAE, of different regression models $\hat{QoE}=g(x_{1},x_{2})$. --kept outliers}
\label{tab:ml-model-fit-mae}
\begin{tabular}{l|c||l|c}
{Models (linear)} &  {MAE} & {Models (non-linear)} &{MAE}\\
\hline
{Linear Regression} &  {0.69} &  {Decision Tree Regr.}    &  {0.65}\\
{Logistic Regression}  &  {0.65} &  {SVR}       &  {0.60} \\
{Ordinal Regression}       &  {\textbf{0.60}} &  {MLP Regression}       &  {\textbf{0.57}}
\end{tabular}
\end{table}

\begin{table}[h]
\centering
\caption{Performance of models (with outliers).}
\label{tab:performance-ordinal}
\begin{tabular}{c|c|c|ccc}
{} &Model & MAE & \multicolumn{3}{c}{prediction error, $|\hat{QoE}-QoE|$:}   \\
{}& {} & {} & {$=0$}& {$=1$}& {$>1$}\\
\hline
\multirow{3}{*}{\rotatebox[origin=c]{90}{GLMs}} 
    & Ordinal & {0.56} & {53\%} & {39\%} & {8\%}\\
    & Linear & {0.62} & {49\%} & {43\%} & {8\%}\\
    & Logistic & {0.58} & {55\%} & {35\%} & {10\%}\\
\hline
\multirow{3}{*}{\rotatebox[origin=c]{90}{Baselines}} 
    &Dummy & {1.25} & {19\%} & {36\%} & {45\%}\\
    & Vanilla-RS & {0.80} & {49\%} & {33\%} & {18\%}\\
\end{tabular}
\end{table}

\begin{table}[h]
\centering
\caption{Weights of features in Ordinal Regression model --with outliers}
\label{table:weights-ordinal}
\begin{tabular}{c|ccc}
Feature $x_{i}$     &  $QoS$ & $Int$ & $\min\{QoS,Int\}$\\
\hline
Weight $w_{i}$     & {0.19} & {0.30} & {0.51}
\end{tabular}

\end{table}

\begin{figure}[h]\centering
\begin{minipage}[t]{\mycustomwidth}
\centering
\includegraphics[width=\mycustomcolumnwidth]{./figures/ML_plots/bestModelHeatmap_outliers.eps}
\caption{\textit{QoE} as a function of \textit{QoS} and user \textit{interest} --with Outliers.}
\label{fig:model-heat-backup}
\end{minipage}
\hspace{0.05\linewidth}
\begin{minipage}[t]{\mycustomwidth}
\centering
\includegraphics[width=\mycustomcolumnwidth]{./figures/ML_plots/bestModelHeatmap_diff1_outliers.eps}
\caption{ Accuracy of Predictive \textit{QoE} model with +/- 1 distance from true target --with Outliers.}
\label{fig:model-accuracy-diff1}
\end{minipage}
\end{figure}

\section{Analysis QoE grouped as high/low}

\joao{\myitem{An alternative approach to the modelling.} 
Let us recall that each original feature (QoS, Ind, QoR), and the original response QoE, can take integer values from 1 to 5.
For each one of these three original features, we created a new binary feature which can be “Low”, if the original feature is at most 3; or “High”, if the original feature is at least 4. The same procedure was also applied to the response QoE. Therefore, we got three binary features and a binary response. 
A preliminary statistical analysis of the data, based on building contingency tables and computing the chi-square test statistic for pairwise independence, showed that:
\begin{itemize}
  \item 	Regarding their separate predictive power for QoE, QoS is the strongest feature (Chi-square = 137.77), followed by Interest (Chi-square = 117.22) and QoR (Chi-square = 43.91).
\item	Fortunately, all three features are weakly related to each other: Chi-square(QoS, Int) = 26.55,  Chi-square(QoS, QoR) = 6.22, Chi-square(QoR, Int) = 23.87.
\item	Considering the dependence relationship between a pair of features and QoE, we got: Chi-square[(QoS, Int), QoE] = 223.16, Chi-square[(QoS, QoR), QoE] = 167.01, Chi-square[(QoR, Int), QoE] = 135.57. Then, (QoS, Int) seems to be the most promising pair of features for predicting QoE.
\end{itemize}
Our final goal here was to build a classifier, namely, a rule capable of predicting whether QoE would be High or Low, given:
\begin{itemize}
\item	A combination of the input binary features (e.g., QoS = High, Int = Low, QoR = High);
\item	The overall proportion of High QoE sessions in the target population.
\end{itemize}
Our results are summarized in the following table, where:
\begin{itemize}
\item The three first columns indicate each one of the eight possible input feature combinations.
\item The labels on top of the remaining columns indicate the overall proportion of High QoE sessions, varying from 0.1 to 0.9.
\item The contents of these remaining columns indicate the predicted QoE (Low or High).
\end{itemize}
\begin{center} 
\begin{tabular}{| c | c | c || c | c | c | c | c | }
\hline
 QoS & Int & QoR & 0.1 & 0.2 & 0.3 & 0.4 & 0.5 \\ 
 \hline
 Low & Low & Low & Low & Low & Low & Low & Low \\  
 Low & Low & High & Low & Low & Low & Low & Low \\
 Low & Low & High & Low & Low & Low & Low & Low \\
 Low & High & High & Low & Low & Low & Low & Low \\
 High & Low & Low & Low & Low & Low & Low & Low \\
 High & Low & High & Low & Low & Low & Low & High \\
 High & High & Low & Low & Low & High & High & High \\
 High & High & High & High & High & High & High & High \\   
 \hline
 QoS & Int & QoR & 0.6 & 0.7 & 0.8 & 0.9 & \\
 \hline
 Low & Low & Low & Low & Low & Low & Low & \\  
 Low & Low & High & Low & Low & Low & Low & \\
 Low & Low & High & Low & Low & Low & High & \\
 Low & High & High & High & High & High & High & \\
 High & Low & Low & Low & Low & High & High & \\
 High & Low & High & High & High & High & High & \\
 High & High & Low & High & High & High & High & \\
 High & High & High & High & High & High & High & \\
\hline
\end{tabular}
\end{center}
In order to build this classifier from the available dataset, we used a statistical methodology based on a Naïve Bayes approach. The procedure assumes that the binary features are conditionally independent, given the binary response.
The classifier accuracy was estimated by cross-validation to be 86\%, if the overall proportion of High QoE sessions is around 50\% (the one prevailing in our dataset). 
}

\section{Some extra material}

\daniel{the click rate for the nudged system remains the same, even though we changed the order of items, i.e., click rate is quite robust/insensitive against ordering}

\daniel{message: by changing recommendations, we are not changing too much the quality of recommendations;  changing ranking: doing better than blue is a bit cheating? we are tilting the order;
being on top of blue curve, does not mean we are beating the Youtube recommendation:  it means that changing  position there are potential gains without significantly costs }

\joao{I understand that each observation in the dataset corresponds to a user watching a video. So, each user can be present in at most 5 observations. Is that right?
How many observations do we have altogether?
Since the goal here is to improve QoE, it seems to me that trying to fit a regression model with QoE as the response and: Interest, QoS, QoR (and perhaps a dummy 0-1 variable for cache) as possible features could be a good idea. Felipe suggested something like this in a recent chat. My only concern about this approach is that, according to the theory of Regression Analysis, the response variable should be continuous. And QoE is discrete, with only 6 possible values: integers from 0 to 5, right? One possible way to circumvent this issue could be previously adding a small variance random noise to QoE, as we did in some parts of our recent article.
My hope is that this regression fit could help us quantifying the effect of each possible feature (Interest, QoS, QoR and the cache dummy variable) on QoE.}

The number of participants per region is given in Table~\ref{table:number-of-participants}.

\begin{table}[h]
    \centering
    \caption{Number of participants per region.}
    \label{table:number-of-participants}
    \begin{tabular}{l|ccccc|c}
         \textbf{\textit{Regions}}            &  Greece & Brazil & France & US & India & TOTAL\\
         \textbf{\textit{\# participants}}    & \red{630} &\red{61} &\red{28} &\red{17} &\red{3} &\red{739}
    \end{tabular}
\end{table}

Table~\ref{tab:interest-ratings-pmf} shows the distribution of the \textit{Interest} ratings for the low-QoS and high-QoS videos. The interest for contents from initial YouTube recommendations (i.e., all low-QoS videos) is only slightly higher than for contents recommended by the QoS-aware algorithm; see for example that low-QoS videos have more ratings with 4 or 5 stars and less for 1 or 2 stars. This indicates that \textit{biasing recommendations towards high-QoS content, does not have a significant negative impact in user interest}. 
\begin{table}[h]
\centering
\caption{Number of responses per \textit{Interest} rating}
\label{tab:interest-ratings-pmf}
\begin{tabular}{l|ccccc}
{} & \multicolumn{5}{c}{{Rating of \textit{Interest}}}\\
\textbf{\#Responses}       & {1}$\bigstar$ & {2}$\bigstar$ &{3}$\bigstar$ &{4}$\bigstar$ &{5}$\bigstar$ \\
\hline 
% {Low-QoS videos} &  17  & 34 &  41 & 65 & 58 \\
% {High-QoS videos} &  40 &  38 & 58 & 72 & 106
{Low-QoS videos} &  ~8\% &   16\% &   19\% & 30\% &   27\% \\
{High-QoS videos} & 13\% &   12\% &   18\% &   23\% &   34\%
\end{tabular}
\end{table}

\myitem{Figure~\ref{fig:chrcrr-vs-5}} presents the average CHR (blue bars) and CRR (red bars) values per step in an experiment session. The decrease in the CRR is due to the caching policy we considered (control variable). We can observe that the CHR values follow the CRR values, which means that the users are equally probable to select cached contents (which are typically favored by the QoS-aware recommendations) and not-cached contents (which are from the initial YouTube recommendations). This indicates that \textit{using a carefully designed QoS-aware RSs does not have a negative impact on user preferences}.

\myitem{Figure~\ref{fig:qor-vs-interest}} shows the CDF of ratings for Interest and QoR. \pavlos{@Savvas: is this plot only for cached contents?} \savvas{@pavlos: no, for all samples.} On average, the Interest ratings are slightly higher than the QoR ratings, which indicates even if a user is sometimes not very satisfied by a biased recommendation list, ultimately, he can still select a content that satisfies him.

\myitem{Figure~\ref{fig:chr-vs-int-qor}} shows that the CHR decreases as the ratings of users become higher. However, this plot still verifies that the final interest is higher than the perception of the user for the recommendations. \pavlos{I'm not sure (i) if this explanation makes much sense, (ii) whether we should present in a different way these results, or (iii) not present them at all.}

\begin{figure}[h]\centering
\begin{minipage}[t]{0.46\linewidth}
\centering
\includegraphics[width=1\columnwidth]{./figures/figuresSavvas/qorsoifixed.eps}
\caption{QoR with Sum Of Indexes}
\label{fig:qor-vs-soi}
\end{minipage}
\begin{minipage}[t]{0.46\linewidth}
\centering
\includegraphics[width=1\columnwidth]{./figures/figuresSavvas/intsoi.eps}
\caption{Interest with Sum Of Indexes}
\label{fig:int-vs-soi}
\end{minipage}
\end{figure}

\begin{figure}[h]\centering
\begin{minipage}[t]{0.46\linewidth}
\centering
\includegraphics[width=1\columnwidth]{./figures/figuresSavvas/chrcrrfixed.eps}
\caption{CHR, CRR in 4 consequent video sessions}
\label{fig:chrcrr-vs-5}
\end{minipage}
\begin{minipage}[t]{0.46\linewidth}
\centering
\includegraphics[width=1\columnwidth]{./figures/figuresSavvas/cdf_intNext_qorPrev.eps}
\caption{QoR x Interest }
\label{fig:qor-vs-interest}
\end{minipage}
\end{figure}

\newpage 

\begin{figure}[h]\centering
\begin{minipage}[t]{0.46\linewidth}
\centering
\includegraphics[width=1\columnwidth]{./figures/figuresSavvas/qorsoibuckets.eps}
\caption{QoR with Sum Of Indexes - Buckets}
\label{fig:qor-vs-soi-buckets}
\end{minipage}
\begin{minipage}[t]{0.46\linewidth}
\centering
\includegraphics[width=1\columnwidth]{./figures/figuresSavvas/intsoibuckets.eps}
\caption{Interest with Sum Of Indexes - Buckets}
\label{fig:int-vs-soi-buckets}
\end{minipage}
\end{figure}

\begin{figure}[h]\centering
\begin{minipage}[t]{0.46\linewidth}
\centering
\includegraphics[width=1\columnwidth]{./figures/figuresSavvas/abandonment.eps}
\caption{Ratings in Abandoned Video Sessions}
\label{fig:abandonment}
\end{minipage}
\begin{minipage}[t]{0.46\linewidth}
\centering
\includegraphics[width=1\columnwidth]{./figures/figuresSavvas/chrXqorXint.eps}
\caption{Fraction of Cached Contents based on Ratings}
\label{fig:chr-vs-int-qor}
\end{minipage}
\end{figure}

\begin{figure}[h]\centering
\begin{minipage}[t]{0.46\linewidth}
\centering
\includegraphics[width=1\columnwidth]{./figures/figuresSavvas/cdf_interest.eps}
\caption{CDF(Interest) for Cached, Non Cached \pavlos{added as Table/text}}
\label{fig:cdf-vs-interest}
\end{minipage}
\begin{minipage}[t]{0.46\linewidth}
\includegraphics[width=1\columnwidth]{./figures/ML_plots/intVSqos_ORD_split_80_20_keep_outliers.eps}
\caption{ QoE predictions of MLP regression model with features QoS and Int. --kept outliers}
\label{fig:mlp-kept-outliers}

\end{minipage}

\begin{minipage}[t]{1\linewidth}
\centering
\includegraphics[width=1\columnwidth]{./figures/ML_plots/prevQoRvsInt_classes.eps}
\caption{ Interest Ratings Ratio over QoR Ratings}
\label{fig:prevQoRvsInt_samplesNum}

\end{minipage}
\end{figure}

\begin{table}[h]
\centering
\caption{Chi-squared test, null assumption ``QoE is independent from X'' (X$\in$ \{QoS, QoR, Interest\}); The null assumption is always rejected with the presented p-values. }
\label{tab:chi-squared-tests}
\begin{tabular}{c|c}
     {X}& {p-value}  \\
     \hline
     {QoS}& {$1.47\cdot 10^{-54}$} \\
     {QoR}& {$7.90\cdot 10^{-38}$} \\
     {Interest}& {$6.32\cdot 10^{-43}$} \\
\end{tabular}
\end{table}
